# Supplementary material for: Simplicial 2-Complex Convolutional Neural Nets
Source: arXiv:2012.06010 source file (2020-12-10)
Supplement: Supplementary file 1 [file appendix.tex]

\appendix
\input{learning_ph}
